# Supplementary material for: Learning Multiple Visual Tasks while Discovering their Structure
Source: arXiv:1504.03106 source file (2015-04-13)
Supplement: Supplementary file 1 [file egpaper_for_review_supplementary_material.pdf]

## 6. Supplementary Material

### 6.1. On the (joint) convexity of Sparse Kernel MTL

As stated in the paper, the Sparse Kernel MTL problem is jointly convex in the two optimization variables. The proof of this fact is an extension of similar results in [2, 23] and we give it here for completeness.

**Proposition 6.1.** *Let  $V : \mathbb{R}^T \rightarrow \mathbb{R}^T \rightarrow \mathbb{R}_+$  be a convex loss function. Then the functional in problem (4) is convex in both  $f$  and  $A$ .*

*Proof.* Notice that, the only term that requires some care is the component of the functional that is mixing  $f$  and  $A$  together, namely  $\|f\|_{\mathcal{H}}$  (where the dependency to  $A$  is implicit in  $\mathcal{H}$ ). Indeed, since  $V$  is chosen to be convex, the empirical risk term is clearly convex in  $f$  and does not depend on  $A$ , while all the remaining terms are – i.e. the  $\text{tr}(A^{-1})$ ,  $\text{tr}(A)$  and  $\|A\|_{\ell_1}$  – penalize only the structure matrix  $A$  and are clearly convex with respect to it.

According to equation (6), we have seen that we can actually restrict our problem to functions  $f(\cdot) = \sum_{i=1}^n k(\cdot, x_i) b_i$  with  $b_i \in \mathbb{R}^T$  and that  $\|f\|_{\mathcal{H}}^2$  can be rewritten as  $\|f\|_{\mathcal{H}}^2 = \text{tr}(B^T K B A^{-1})$ , with  $K \in S_+^n$  the empirical kernel matrix. Let us know set  $b = \text{vec}(B) \in \mathbb{R}^{nT}$  the vectorization of matrix  $B$ , obtained by concatenating the columns of  $B$ . Then we have that

$$\text{tr}(B^T K B A^{-1}) = b^T (A^{-1} \otimes K) b. \quad (11)$$

In order to show that the function  $Q(A, b) = b^T (A^{-1} \otimes K) b$  is jointly convex in  $b$  and  $A$  we will show that its epigraph is a convex set. To see this notice that

$$\begin{aligned} \text{epi}_Q &= \{(A, b, c) \in S_{++}^T \times \mathbb{R}^{nT} \times \mathbb{R} \mid c \geq w^T (A^{-1} \otimes K) w\} \\ &= \{(A, b, c) \in S_{++}^T \times \mathbb{R}^{nT} \times \mathbb{R} \mid \begin{pmatrix} A \otimes K^\dagger & b \\ b^T & c \end{pmatrix} \in S_{++}^{nT+1}\} \end{aligned} \quad (12)$$

where the second equality is directly derived from a Schur's complement argument. Consider now any couple of points  $(A_1, b_1, c_1), (A_2, b_2, c_2) \in \text{epi}_Q$  and any  $\theta \in [0, 1]$ . We clearly have that the convex combination

$$\begin{aligned} &\theta \begin{pmatrix} A_1 \otimes K^\dagger & b_1 \\ b_1^T & c_1 \end{pmatrix} + (1 - \theta) \begin{pmatrix} A_2 \otimes K^\dagger & b_2 \\ b_2^T & c_2 \end{pmatrix} \\ &= \begin{pmatrix} \theta A_1 \otimes K^\dagger + (1 - \theta) A_2 \otimes K^\dagger & \theta b_1 + (1 - \theta) b_2 \\ \theta b_1^T + (1 - \theta) b_2^T & \theta c_1 + (1 - \theta) c_2 \end{pmatrix} \end{aligned} \quad (13)$$

still belongs to  $S_{++}^{nT+1}$ , which implies that

$$(\theta A_1 + (1 - \theta) A_2, \theta b_1 + (1 - \theta) b_2, \theta c_1 + (1 - \theta) c_2) \in \text{epi}_Q \quad (14)$$

therefore proving that  $Q$  is jointly convex in  $b$  and  $A$ .  $\square$

### 6.2. Cluster Multi-task Learning

We briefly recall here the Convex Multi-task Cluster Learning proposed in [11] and show that it can be cast in the same framework as that of our Sparse Kernel MTL model. In particular we comment what choice of constraint set  $\mathcal{A}$  can be imposed on the structure matrix  $A$  to recover clustered structures of tasks.

In the setting proposed by [11], tasks are assumed to belong to one of  $r$  of unknown clusters, with  $r$  fixed a priori. While the original formulation is for the linear kernel, it can be easily extended to the non-linear setting of RKHSv. Let  $E \in \{0, 1\}^{T \times r}$  be the binary matrix whose entry  $E_{st}$  has value 1 whenever a task  $s$  belongs to cluster  $t$ , and 0 otherwise. Let  $L$  be the normalized Laplacian of the Graph defined by  $E$ . Set  $M = I - L$ , and  $U = \frac{1}{T} 11^\top$ . As we have observed in Eq. (6), the regularizer  $\|f\|_{\mathcal{H}}$  depends on  $A^{-1}$ . The role of this term could be shaped to reflect the structure of the clusters encoded in the Laplacian  $L$ , hence in the matrix  $M$ . As noted in [11]  $A^{-1}(M)$  can be chosen so that:

$$A^{-1}(M) = \epsilon_M U + \epsilon_B (M - U) + \epsilon_W (I - M), \quad (15)$$

where the first term is a global penalty on the average predictor, the second term penalizes the between cluster variance, and the third term penalizes the within cluster variance. Since  $M$  belongs to a discrete set, the authors propose a relaxation for  $M$  by constraining it to be in a convex set  $\mathcal{S}_c = \{M \in S_+^T, 0 \preceq M \preceq I, \text{tr}(M) = r\}$  which directly induces a set  $\mathcal{A}$  of spectral constraints for  $A$ .

## 7. Further Results

We report here further results that suggest the efficacy of our method in sharing information across tasks also in settings that are not related to computer vision applications. While the interpretation of the sparse matrix recovered was less clear in this context, we notice that such recovered structure is beneficial to the multi-task prediction.

**Sarcos.** Sarcos<sup>3</sup> is a regression dataset designed to evaluate machine learning solutions for inverse dynamics problems in robotics. It consists in a collection of 21-dimensional inputs, i.e. the joint positions, velocities and acceleration of a robotic arm with 7 degrees of freedom and 7 outputs (the tasks), which report the corresponding torques measured at each joint.

For each task, we randomly sampled 50, 100, 150 and 200 training examples while we kept a test set of 5000 examples in common for all tasks. We used a linear kernel and performed 5-fold crossvalidation to find the best regularization parameter according to the normalized mean squared

<sup>3</sup>[urlhttp://www.gaussianprocess.org/gpml/data/](http://www.gaussianprocess.org/gpml/data/)

|       | 50 tr. samples per class              |               | 100 tr. samples per class             |               | 150 tr. samples per class             |               | 200 tr. samples per class |        |
|-------|---------------------------------------|---------------|---------------------------------------|---------------|---------------------------------------|---------------|---------------------------|--------|
|       | nMSE ( $\pm$ std)                     | nI            | nMSE ( $\pm$ std)                     | nI            | nMSE ( $\pm$ std)                     | nI            | nMSE ( $\pm$ std)         | nI     |
| STL   | 0.2436 $\pm$ 0.0268                   | 0             | 0.1723 $\pm$ 0.0116                   | 0             | 0.1483 $\pm$ 0.0077                   | 0             | 0.1312 $\pm$ 0.0021       | 0      |
| MTFL  | 0.2333 $\pm$ 0.0213                   | 0.0416        | 0.1658 $\pm$ 0.0107                   | 0.0379        | 0.1428 $\pm$ 0.0083                   | 0.0281        | 0.1311 $\pm$ 0.0055       | 0.0003 |
| MTRL  | 0.2314 $\pm$ 0.0217                   | 0.0404        | 0.1653 $\pm$ 0.0112                   | 0.0401        | 0.1421 $\pm$ 0.0081                   | 0.0288        | 0.1303 $\pm$ 0.0058       | 0.0071 |
| OKL   | 0.2284 $\pm$ 0.0232                   | 0.0630        | 0.1604 $\pm$ 0.0123                   | 0.0641        | <b>0.1410 <math>\pm</math> 0.0087</b> | 0.0350        | 0.1301 $\pm$ 0.0073       | 0.0087 |
| SKMTL | <b>0.2127 <math>\pm</math> 0.0248</b> | <b>0.0713</b> | <b>0.1591 <math>\pm</math> 0.0127</b> | <b>0.0748</b> | <b>0.1410 <math>\pm</math> 0.0081</b> | <b>0.0393</b> | 0.1303 $\pm$ 0.0071       | 0.0073 |

Table 4. Comparison of Multi-task learning methods on the Sarcos dataset. The advantage of learning the tasks jointly decreases as more training examples became available.

error (nMSE) of predicted torques. We averaged the results over 10 repetitions of these experiments. The results, reported in Table 4, show clearly that to adopt a multi-task approach in this setting is favorable; however, in order to quantify more clearly such improvement, we report in Table 4 also the *normalized improvement* (nI) over single-task learning (STL). For each multi-task method MTL, the normalized improvement nI(MTL) is computed as the average

$$\text{nI(MTL)} = \frac{1}{n_{exp}} \sum_{i=1}^{n_{exp}} \frac{\text{nMSE}_i(\text{STL}) - \text{nMSE}_i(\text{MTL})}{\sqrt{\text{nMSE}_i(\text{STL}) \cdot \text{nMSE}_i(\text{MTL})}}$$

over all the  $n_{exp} = 10$  experiments of the normalized differences between the nMSE achieved by respectively the STL approach and the given multi-task method MTL.
